# Supplementary material for: Synchronization of interconnected networks: the role of connector nodes
Source: arXiv:1406.0081 ancillary file (2014-06-04)
Supplement: Supplementary file 1 [file supplemental_material.pdf]

## Supplemental Material. Synchronization of interconnected networks: the role of connector nodes

J. Aguirre, R. Sevilla-Escoboza, R. Gutiérrez, D. Papo, and J. M. Buldú

### S1 Analytical study of the synchronization of a network of networks in an exactly solvable example

#### S1.1 Description of the system: two stars connected by a unique inter-link

To understand the influence of the connector nodes in the synchronization of a network of networks (*NoN*), we have considered the simplest configuration that can be analytically treated: two star networks connected by one single inter-link. Each star consists of  $N$  nodes, one high-degree node (H) connected to  $N - 1$  low-degree nodes (L). All links inside each star have the same weight. The topology is thus characterized by a weighted adjacency matrix  $\mathbf{W} = \{w_{ij}\}$  such that  $w_{ij} = w_{intra}$  if  $i$  and  $j$  are connected nodes from the same star,  $w_{ij} = w_{inter} = aw_{intra}$  if  $i$  and  $j$  are connector nodes, each of them from a different star, and  $w_{ij} = 0$  if  $i$  and  $j$  are not connected. The elements of the Laplacian matrix  $\mathbf{L} = \{l_{ij}\}$  are  $l_{ij} = \delta_{ij}(\sum_{k=1}^N w_{ik}) - w_{ij}$ , where  $\delta_{ij}$  denotes the Kronecker delta. The eigenvalues are denoted  $0 = \lambda_1 < \lambda_2 \leq \dots \leq \lambda_N$ ,  $\lambda_2$  and  $\lambda_N$  determining the synchronizability of the system. To simplify the expressions shown here, we have fixed  $w_{intra} = 1$ . Considering  $w_{intra} \neq 1$  would require multiplying the eigenvalues of the Laplacian matrix by  $w_{intra}$ , but the phenomenology would be qualitatively identical.

Three connecting strategies are used: HH (the high-degree node of one network with its counterpart in the other network), HL (the high-degree node of one network with a low-degree node of the other network), and LL (a low-degree node of one network with a low-degree node of the other network).

#### S1.2 Eigenvalues of the Laplacian matrix associated to the system

The symmetry of the configuration simplifies the characteristic polynomial of the Laplacian matrix. As a result,  $\lambda_N$  and  $\lambda_2$  are respectively, and for all  $N$  and  $a$ , the maximum and minimum roots of Eq. 1 of the main text. The HH case allows even further reduction, as shown in Table S1 and in Eq. 2 of the main text.

| Strategy | $\lambda_N$                                                |
|----------|------------------------------------------------------------|
| HH       | $N/2 + a + \sqrt{(N/2)^2 + a^2 + (N-2)a}$                  |
| HL       | $MaxRoot[x^3 - (1 + N + 2a)x^2 + (N + 2a + aN)x - 2a = 0]$ |
| LL       | $MaxRoot[x^3 - (1 + N + 2a)x^2 + (N + 2aN)x - 2a = 0]$     |
| Strategy | $\lambda_2$                                                |
| HH       | $N/2 + a - \sqrt{(N/2)^2 + a^2 + (N-2)a}$                  |
| HL       | $MinRoot[x^3 - (1 + N + 2a)x^2 + (N + 2a + aN)x - 2a = 0]$ |
| LL       | $MinRoot[x^3 - (1 + N + 2a)x^2 + (N + 2aN)x - 2a = 0]$     |

**Table S1. Largest eigenvalue  $\lambda_N$  and second eigenvalue  $\lambda_2$  of the Laplacian matrix associated to the system.**

The rest of the eigenvalues are, for HH,  $\lambda_{N-1} = N$ ,  $\lambda_{N-2} = \dots = \lambda_3 = 1$  and  $\lambda_1 = 0$ , and, for LL,  $\lambda_{N-1} = N$ ,  $\lambda_{N-2} = 2nd\ Root[x^3 - (1 + N + 2a)x^2 + (N + 2aN)x - 2a = 0]$ ,  $\lambda_{N-3} = \dots = \lambda_3 = 1$  and  $\lambda_1 = 0$ .

| Strategy | $\lambda_N(N \rightarrow \infty)$ | $\lambda_N(a \rightarrow \infty)$ |
|----------|-----------------------------------|-----------------------------------|
| HH       | $N + 2a + O(N^{-1})$              | $2a + N + 1 + O(a^{-1})$          |
| HL       | $N + a + O(N^{-1})$               | $2a + \frac{N}{2} + O(a^{-1})$    |
| LL       | $N + O(N^{-2})$                   | $2a + 1 + O(a^{-1})$              |

  

| Strategy | $\lambda_2(N \rightarrow \infty)$   | $\lambda_2(a \rightarrow \infty)$                                                                             |
|----------|-------------------------------------|---------------------------------------------------------------------------------------------------------------|
| HH       | $2aN^{-1} + O(N^{-2})$              | $1 + \frac{1-N}{2}a^{-1} + O(a^{-2})$                                                                         |
| HL       | $\frac{2a}{1+a}N^{-1} + O(N^{-2})$  | $\frac{1}{2} + \frac{N-A}{4} + \left( \frac{-N^2+2N-4}{16} + \frac{N^3-8N+8}{16A} \right) a^{-1} + O(a^{-2})$ |
| LL       | $\frac{2a}{1+2a}N^{-1} + O(N^{-2})$ | $\frac{N-B}{2} + \frac{N-2-B}{4B}a^{-1} + O(a^{-2})$                                                          |

**Table S2.** Behavior for large number of nodes per network  $N$  and large inter-link weight  $a$  of the largest eigenvalue  $\lambda_N$  and second eigenvalue  $\lambda_2$  of the Laplacian matrix associated to the system. To simplify the mathematical expressions, we have used  $A = \sqrt{N^2 + 4N - 12}$  and  $B = \sqrt{N^2 - 4}$ .

| Strategy | $r(N \rightarrow \infty)$                                                                              |
|----------|--------------------------------------------------------------------------------------------------------|
| HH       | $\frac{N^2}{2a} + 2N + 2a - 2 + O(N^{-2})$                                                             |
| HL       | $\frac{1+a}{2a}N^2 + \frac{a^2+4a+1}{2(1+a)}N + \frac{a^5+5a^4+2a^3-6a^2-11a-3}{2(1+a)^3} + O(N^{-1})$ |
| LL       | $\frac{1+2a}{2a}N^2 - \frac{N}{1+2a} - \frac{8a^3+12a^2+8a+1}{(1+2a)^3} + O(N^{-1})$                   |

  

| Strategy | $r(a \rightarrow \infty)$                                                           |
|----------|-------------------------------------------------------------------------------------|
| HH       | $2a - 2 + 2N + O(a^{-1})$                                                           |
| HL       | $\frac{8}{2+N-A}a + \frac{-4N^3-8N^2+40N-16+(8+4N^2)A}{2+N+A(2+N-A)^2} + O(a^{-1})$ |
| LL       | $\frac{4}{N-B}a + \frac{-2N^2-N+12+(N+2)B}{B(N-B)^2} + O(a^{-1})$                   |

**Table S3.** Behavior for large number of nodes per network  $N$  and large inter-link weight  $a$  of the ratio between the largest eigenvalue  $\lambda_N$  and the second eigenvalue  $\lambda_2$  of the Laplacian matrix associated to the system.  $A$  and  $B$  as in caption of Table S2.

### S1.3 Analytic derivations associated to the system of two star networks connected by a unique inter-link

#### S1.3.1 The eigenratio $r$ for the different connecting strategies

In this Section we investigate which connecting strategy leads to the lowest eigenratio  $r$ , that is, synchronizes the best. For small values of  $aN$ , we make use of the fact that Eq. 1 of the main text only differs in  $C_1$  for the HH, LL and HL strategies. We can express  $C_1^{\text{HL}}$  as a perturbation of  $C_1^{\text{HH}}$ , and  $\lambda_N^{\text{HL}}$  and  $\lambda_2^{\text{HL}}$  as perturbations of  $\lambda_N^{\text{HH}}$  and  $\lambda_2^{\text{HH}}$  respectively, obtaining

$$r^{\text{HL}} = \frac{\lambda_N^{\text{HL}}}{\lambda_2^{\text{HL}}} = \frac{\lambda_N^{\text{HH}} + \Delta\lambda_N}{\lambda_2^{\text{HH}} + \Delta\lambda_2} \sim r^{\text{HH}} + r^{\text{HH}} \left( \frac{\Delta\lambda_N}{\lambda_N^{\text{HH}}} - \frac{\Delta\lambda_2}{\lambda_2^{\text{HH}}} \right). \quad (\text{S1})$$

In consequence, the sign of  $(\Delta\lambda_N/\lambda_N^{\text{HH}} - \Delta\lambda_2/\lambda_2^{\text{HH}})$  defines whether  $r^{\text{HH}}$  or  $r^{\text{HL}}$  is larger. From Eq. 1 of the main text we obtain for the HL strategy

$$x^3 + C_2x^2 + (C_1^{\text{HH}} + \epsilon)x + C_0 = 0, \quad (\text{S2})$$

where  $\epsilon = a(N - 2)$ . Introducing  $\lambda_{N,2}^{\text{HH}} + \Delta\lambda_{N,2}$  in Eq. S2, and disregarding terms of second and third order for  $\Delta\lambda_{N,2}$ , we obtain

$$\frac{\Delta\lambda_{N,2}}{\lambda_{N,2}^{\text{HH}}} = -\frac{\epsilon}{3(\lambda_{N,2}^{\text{HH}})^2 + 2C_2\lambda_{N,2}^{\text{HH}} + C_1^{\text{HH}} + \epsilon}. \quad (\text{S3})$$

This yields

$$\Delta\lambda_N/\lambda_N^{\text{HH}} - \Delta\lambda_2/\lambda_2^{\text{HH}} > 0 \Leftrightarrow 3(\lambda_N^{\text{HH}})^2 + 2C_2\lambda_N^{\text{HH}} > 3(\lambda_2^{\text{HH}})^2 + 2C_2\lambda_2^{\text{HH}}. \quad (\text{S4})$$

Let us see for which values of the parameters  $N$  and  $a$  the right-hand side of Eq. S4 is satisfied. The polynomial  $3\lambda^2 + 2C_2\lambda$  crosses the X-axis in  $\lambda = 0$  and  $\lambda = -2C_2/3$ . Therefore, as  $\lambda_N^{\text{HH}} > \lambda_2^{\text{HH}} > 0$ , verifying that  $\lambda_N^{\text{HH}} > -2C_2/3$  implies that  $3\lambda_N^2 + 2C_2\lambda_N > 3\lambda_2^2 + 2C_2\lambda_2$ . Taking  $C_2 = -(1 + N + 2a)$  and  $\lambda_N^{\text{HH}}$  from Eq. 2 of the main text, we obtain

$$\lambda_N^{\text{HH}} > -2C_2/3 \Leftrightarrow N^2 + 4a + (4N - 11)a - 1 > 0. \quad (\text{S5})$$

As the right-hand side of Eq. S5 is satisfied for all meaningful values of  $N$  and  $a$ , it results that  $\Delta\lambda_N/\lambda_N - \Delta\lambda_2/\lambda_2 > 0$  and therefore  $r^{\text{HL}} > r^{\text{HH}} \forall (N > 2, a > 0)$ . The same argument for  $r^{\text{LL}}$  as a perturbation of  $r^{\text{HL}}$  implies

$$r^{\text{HH}} < r^{\text{HL}} < r^{\text{LL}} \forall (N > 2, a > 0), \quad (\text{S6})$$

thus, proving that the HH strategy is the one that promotes the most the synchronizability of the  $NoN$ , while the LL strategy is the worst possible one.

A different argument that can be applied for high values of  $N$  is the following. The analytical expression for  $r^{\text{HL}} = \lambda_N^{\text{HL}}/\lambda_2^{\text{HL}}$  from the equations of Table S1 is too complex to work with it, but we can do  $r^{\text{HH}}(N \rightarrow \infty) = r^{\text{HL}}(N \rightarrow \infty)$ , neglecting terms of order  $O(N^{-1})$ , to find the values of  $N$  and  $a$  for which both curves intersect for large networks:

$$N = \frac{3 + 6a + 2a^2 - 2a^3 - a^4 \pm \sqrt{5 + 36a + 96a^2 + 140a^3 + 126a^4 + 60a^5 - 12a^7 - 3a^8}}{2(a^3 + 3a^2 + 3a + 1)}. \quad (\text{S7})$$

This expression yields that  $N < 3 \forall a$ , implying that  $r^{\text{HH}}$  and  $r^{\text{HL}}$  never cross for realistic systems and in consequence  $r^{\text{HL}} > r^{\text{HH}} \forall (N > 2, a > 0)$ .

### S1.3.2 Determining the minima of the eigenratio $r$ for the different connecting strategies

As  $\lim_{a \rightarrow \infty} r^{\text{HH,HL,LL}} = \infty$  and  $\lim_{a \rightarrow 0} r^{\text{HH,HL,LL}} = \infty \forall N > 2$ , there exists (at least) one critical value of the weights  $a_{\text{sync}}^{\text{HH}}$ ,  $a_{\text{sync}}^{\text{HL}}$  and  $a_{\text{sync}}^{\text{LL}}$  such that  $r^{\text{HH}}$ ,  $r^{\text{HL}}$  and  $r^{\text{LL}}$  respectively are minimum and therefore the synchronizability is optimum.

Furthermore, let us prove that the minimum values for  $r^{\text{HH}}$ ,  $r^{\text{HL}}$  and  $r^{\text{LL}}$  for a fixed value of  $N$  do not coincide at the same value of the weight  $a$ . For the HH strategy, we see that

$$dr^{\text{HH}}/da = 0 \Rightarrow a_{\text{sync}}^{\text{HH}} = N/2, \quad (\text{S8})$$

where the expression of  $r^{\text{HH}}$  was obtained using the explicit expressions of  $\lambda_N$  and  $\lambda_2$  shown in Table S1. For the HL case these expressions are much more complex, but we can do

$$dr^{\text{HL}}(N \rightarrow \infty)/da = 0 \Rightarrow$$

$$N = F(a_{sync}^{HL}) = \frac{3a^2 + 8a^3 + 8a^4 + 4a^5 + a^6 + a(1+a)^2\sqrt{-8 + 40a + 57a^2 + 92a^3 + 50a^4 + 12a^5 + a^6}}{2 + 8a + 12a^2 + 8a^3 + 2a^4}, \quad (S9)$$

where we have neglected terms of order  $O(N^{-1})$  in  $r^{HL}(N \rightarrow \infty)$ . It is clear that there is no explicit expression for  $a_{sync}^{HL}$  as a function of  $N$ , but we can do the following to compare  $a_{sync}^{HH}$  and  $a_{sync}^{HL}$ : For every value of  $N$ , we obtain

$$N = 2a_{sync}^{HH} = F(a_{sync}^{HL}) \Rightarrow a_{sync}^{HH} > a_{sync}^{HL} \Leftrightarrow \frac{F(a_{sync}^{HL})}{2} > a_{sync}^{HL}. \quad (S10)$$

Substituting Eq. S9 in Eq. S10, we see that the right-hand side of the latter is satisfied for every  $a_{sync}^{HL} > 0.55$  and therefore for every  $N > 1.1$ . In conclusion, the optimum value of the weight  $a$  for synchronizing the HH case is always larger than the optimum value for the HL case, that is,  $a_{sync}^{HH} > a_{sync}^{HL}$  for all values of the size of the networks  $N$ .

## S2 Dependence of synchronizability of two coupled generic networks on the size of the networks

As mentioned in the main text,  $\lambda_2$  determines the synchronizability of class II systems [17]. From a network perspective,  $\lambda_2$  is a measure of the modularity, in such a way that the smaller  $\lambda_2$ , the more modular a network is and therefore the harder it is to synchronize [29]. When considering a network-of-networks,  $\lambda_2$  is also an indicator of the existence of modules, in this case, each one corresponding to a sub-network with its own identity. This way, we can heuristically see that, for a given average connectivity, the size of the sub-networks hinders synchronizability with the following reasoning: If we add nodes to two connected networks linked with a unique inter-link, the system will have more nodes and more intra-links, but still only one inter-link, becoming more modular, that is, reinforcing the sub-networks (i.e., modules) and facilitating the decomposition of the network-of-networks into modules. In the limit  $N \rightarrow \infty$ ,  $\lambda_2 \rightarrow 0$ , as it is known that  $\lambda_2 = 0$  is the condition for a network to be partitioned [29] and MSF arguments dictate that synchronization becomes necessarily unstable. In conclusion, adding nodes to the networks implies less  $\lambda_2$  and therefore hinders synchronizability.

In the case of class III systems, synchronizability depends on  $r = \lambda_N/\lambda_2$ , in such a way that the lower  $r$ , the more synchronizable the system is. According to [39–41],

$$\frac{N}{N-1}k_{\max} \leq \lambda_N \leq 2k_{\max}, \quad (S11)$$

from where we obtain that

$$\frac{N}{N-1} \frac{k_{\max}}{\lambda_2} \leq r \leq 2 \frac{k_{\max}}{\lambda_2}. \quad (S12)$$

For a given average connectivity, and except for very pathological cases, increasing the size of a network makes its maximum degree  $k_{\max}$  increase or, at the very least, remain constant, and as we have seen that  $\lambda_2 \rightarrow 0$  when  $N \rightarrow \infty$ , Eq. S12 yields that  $r$  is on average expected to grow with  $N$  for all cases of interest, thus hindering synchronizability.

Interestingly, the dependence of  $\lambda_N$  on  $N$  is functionally different depending on the topology of the networks, as can be inferred from Fig. 3 of the main text:  $\lambda_N \sim \sqrt{N}$  for SF networks,  $\lambda_N \sim N^\beta$  where  $\beta \ll 1$  for ER networks, and  $\lambda_N \sim N$  for star networks. The relation  $\lambda_N \sim N$  for star networks was proven in Section S1.2.

There is a theoretical argument that supports the expectation that the relation  $\lambda_N \sim \sqrt{N}$  has general validity for networks whose degree is distributed according to  $P(k) \propto k^{-\gamma}$ . To a very good approximation,

this is the case of any  $NoN$  comprising an arbitrary number of interconnected SF networks, since, for a low number of connector nodes, the degree distribution of a  $NoN$  that follow a given degree distribution  $P(k)$  is essentially  $P(k)$  (it is  $P(k)$  plus a very small perturbation).

The scaling of  $k_{\max}$  for such a case can be predicted by the following heuristic argument. The elements in the degree list  $\{k_1, k_2, \dots, k_N\}$  of a network are identically distributed with a probability density function  $P(k) \sim k^{-\gamma}$ , where we assume  $\gamma > 1$ . As different realizations can give rise to quite different degree lists,  $k_{\max} = \max\{k_1, k_2, \dots, k_N\}$  is expected to vary considerably from one concrete network to another in the ensemble, especially when  $N$  is not very large. For this reason we focus on the ensemble average  $\langle k_{\max} \rangle$ . The fact that  $\langle k_{\max} \rangle$  is the average maximum degree implies that the expected number of instances having a degree higher than  $\langle k_{\max} \rangle$  in  $N$  events (i.e. nodes) is some number no larger than 1 (otherwise, on average we would expect the occurrence of some such larger value to happen at least once),

$$N \int_{\langle k_{\max} \rangle}^{\infty} P(k) dk = \mathcal{O}(1). \quad (\text{S13})$$

Up to constant factors, we can then write

$$\int_{\langle k_{\max} \rangle}^{\infty} k^{-\gamma} dk \sim \langle k_{\max} \rangle^{-\gamma+1} \sim N^{-1}, \quad (\text{S14})$$

which gives  $\langle k_{\max} \rangle \sim N^{1/(\gamma-1)}$ . In the case of scale-free networks generated by the Barabási-Albert preferential attachment growth procedure, the exponent has been proven to be  $\gamma = 3$  for  $N \rightarrow \infty$  [42]. Therefore, we expect that in those networks  $\langle k_{\max} \rangle \sim \sqrt{N}$ .

Finally, from Eq. S11 we obtain  $\langle \lambda_N \rangle \sim \sqrt{N}$ , as we wanted to demonstrate.

### S3 Increasing the number of inter-links

The analytical expressions obtained in previous Sections refer to two connected star networks (Section S1), or to networks with complex topologies (Section S2). In all cases both networks were connected through a single (weighted) link. Nevertheless, the same strategies lead to similar outcomes in more general cases, including a larger number of inter-links. Figure S1 shows how two scale-free networks (generated with the Barabási-Albert model [42]) of  $N = 1000$  nodes interact by means of one (a,b), two (c,d) and ten inter-links (e,f). As in the case of Fig. 1 of the main text, the node number is assigned according to its ranking in the degree distribution (i.e., node 1 is the one with the highest degree and node 1000 the one with the lowest) and, whenever several nodes have the same degree, the eigenvector centrality. This way, coordinate  $(i, j)$  of Figs. S1(a)-(b) indicates the value of  $\lambda_2$  (a) and  $r$  (b) in the case of linking node  $i$  of Network A and node  $j$  of Network B. For the case of  $L = 2$  and  $L = 10$  inter-links, coordinate  $(i, j)$  corresponds to the value of  $\lambda_2$  (c,e) and  $r$  (d,f) when the node  $i+k$  of Network A and  $j+k$  of Network B are connected, with  $k = 0, \dots, L-1$ . We can observe how we obtain the same qualitative results in all cases irrespective of the number of inter-links. The strategy to maximize the stability of the synchronized state is, in all cases, the HH connection. Similar results (not shown here) were obtained with Erdős-Rényi random networks. Therefore, the degree of the connector nodes is crucial in the choice of an interconnection strategy also when several inter-links are established between the networks.

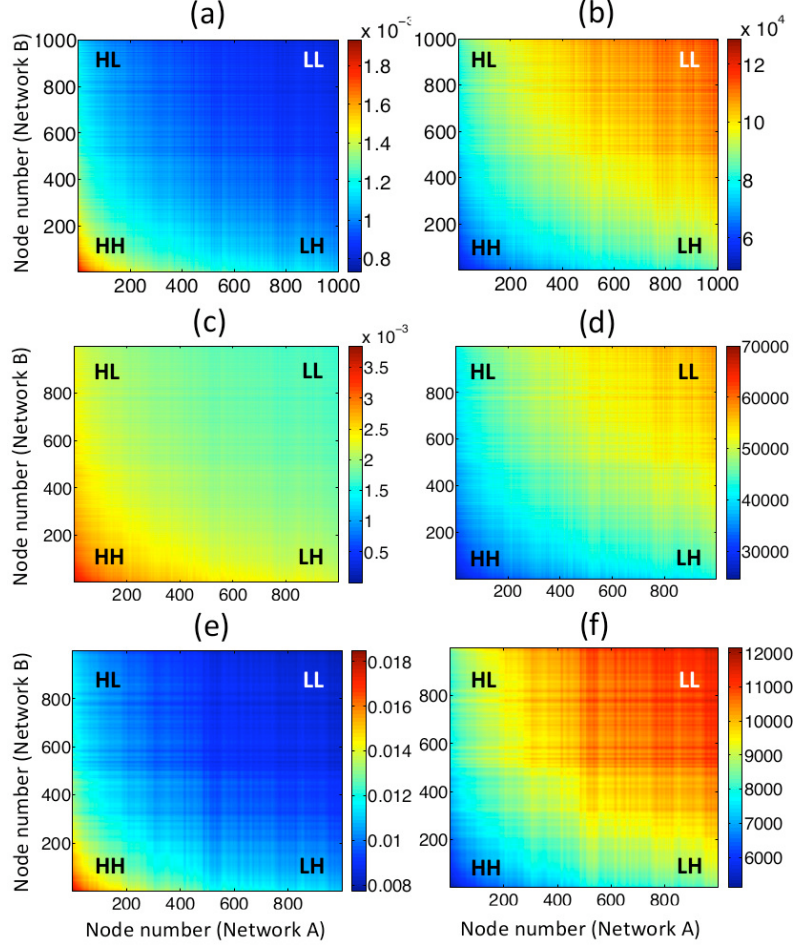

**Figure S1.** (Color online). Interaction between two scale-free networks of  $N = 1000$  nodes. HH corresponds to a strategy connecting high-degree nodes and LL to the connection between low-degree nodes. The value of  $\lambda_2$  is plotted in the left column for different number of inter-links: (a)  $L = 1$ , (c)  $L = 2$  and (e)  $L = 10$ . The right column shows the values of  $r$  for the same number of inter-links. In all cases, HH leads to a higher synchronizability, i.e. the lowest  $\lambda_2$  (for class II systems) and the highest  $r$  (for class III systems). Increasing the number of inter-links leads to the same qualitative behavior.

## S4 Experimental Setup

The robustness of our analytical results is tested with a network of nonlinear electronic circuits. The experimental setup consists of two diffusively coupled star networks ( $N_A = N_B = 6$ ) of piecewise Rössler circuits [31] operating in a chaotic regime [32] (see Fig. S2 for details and Fig. 4 of the main manuscript for the experimental results). Every node (each one being a Rössler-like oscillator circuit) of the  $NoN$  is indexed by  $i = 1, \dots, N_A + N_B$  and it is assigned a three-dimensional state vector  $\mathbf{x}_i(t) \equiv (x_i(t), y_i(t), z_i(t))$ .

Coupling through the  $x$  variable leads to a class III system of equations:

$$\begin{aligned} \dot{x}_i &= -\alpha_i \left[ \Gamma(x_i - \sigma \sum_{j=1}^N w_{ij}(x_j - x_i)) + \beta y_i + \eta z_i \right], \\ \dot{y}_i &= -\alpha_i(-x_i + \gamma y_i), \\ \dot{z}_i &= -\alpha_i(-g(x_i) + z_i), \end{aligned} \quad (\text{S15})$$

where the piecewise part is  $g(x_i) = \mu(x_i - 3)$  if  $x_i > 3$  and zero otherwise,

$$g(x_i) = \begin{cases} 0 & \text{if } x_i \leq 3 \\ \mu(x_i - 3) & \text{if } x_i > 3 \end{cases} \quad (\text{S16})$$

The parameters are:  $\Gamma = 0.05$ ,  $\sigma = 1$ ,  $\beta = 0.5$ ,  $\eta = 1$ ,  $\mu = 15$ , and  $\gamma = 0.02 - \frac{10}{R}$ . We set  $R = 57$   $k\Omega$  to have chaotic dynamics.  $\mathbf{W} = \{w_{ij}\}$  is the weighted adjacency matrix where  $w_{ij} = w_{intra}$  if units  $i$  and  $j$  belonging to the same network are connected,  $w_{ij} = w_{inter}$  if units  $i$  and  $j$  are connected but belong to different networks, and  $w_{ij} = 0$  otherwise.

Interestingly, when coupling is introduced through the  $y$  variable (instead of  $x$ ) we obtain a class II system [35] of equations:

$$\begin{aligned} \dot{x}_i &= -\alpha_i[\Gamma x_i + \beta y_i + \eta z_i], \\ \dot{y}_i &= -\alpha_i(-x_i + \gamma y_i - \sigma \sum_{j=1}^N w_{ij}(y_j - y_i)), \\ \dot{z}_i &= -\alpha_i(-g(x_i) + z_i). \end{aligned} \quad (\text{S17})$$

The schematic representation of the experimental setup is given in Fig. S2. The two star networks A (blue) and B (red) are bidirectionally coupled through an inter-link of weight  $w_{inter}$ . Link weights  $w_{inter}$  and  $w_{intra}$  are adjusted by digital potentiometers X9C104, whose parameters  $C_{u/d}$  (Up/Down resistance) and  $C_{step}$  (increment of the resistance at each step) are controlled by a digital signal coming from the ports P0.0 and P0.3 of a data-acquisition card (DAQ). The twelve output signals were acquired by the analog ports (AI 0; AI 1; ... ; AI 11) of the DAQ Card, and recorded on a computer for further analysis.

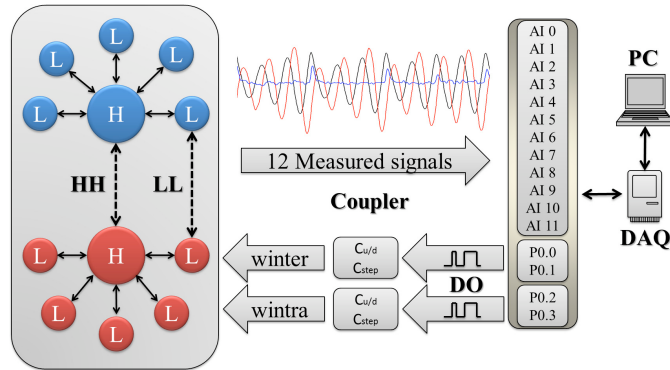

**Figure S2.** (Color online). Experimental setup. Two star networks are bidirectionally coupled by a digital potentiometer X9C104, which sequentially controls the value of  $w_{inter}$  through the digital ports P0.0 and P0.1 of a data-acquisition card. The value of  $w_{intra}$ , accounting for the coupling inside each star network, is controlled by the ports P0.2. and P0.3 of the same card. The  $x$  variable of the  $2 \times N$  Rössler systems is recorded through twelve analog ports (A0.0 to A0.11).

## S5 Master Stability Function of two coupled star networks

We have obtained the Master Stability Function (MSF) [16] of the Rössler systems described in the main text in order to determine the stability of *NoN* synchronization. Given a dynamical system  $i$  whose (uncoupled) dynamics follows  $\dot{\mathbf{x}}_i = \mathbf{F}_i(\mathbf{x}_i)$ , the evolution of  $N$  coupled oscillators (as those in a *NoN*) is given by

$$\dot{\mathbf{x}}_i = \mathbf{F}_i(\mathbf{x}_i) - \sigma \sum_{j=1}^N l_{ij} \mathbf{H}(\mathbf{x}_j), \quad i = 1, \dots, N \quad (\text{S18})$$

where  $\sigma$  is the coupling strength,  $\mathbf{H}(\mathbf{x})$  is a vectorial output function and  $l_{ij}$  are the elements of the Laplacian matrix  $\mathbf{L}$ . For identical systems with the same coupling function  $\mathbf{H}(\mathbf{x})$ , the synchronized state is a solution of  $\dot{\mathbf{x}}_s = \mathbf{F}(\mathbf{x}_s)$  with  $\mathbf{x}_1 = \mathbf{x}_2 = \dots = \mathbf{x}_N \equiv \mathbf{x}_s$ .

When the coupling is introduced through the  $x$  variable (see Eq. S15), the Rössler systems become class III (red circles in Fig. S3) and the MSF has two zeroes, namely  $\nu_1 = 0.107$  and  $\nu_2 = 2.863$ . Both values define the complete synchronization region, since the topology of the network of networks (in our case, two coupled star networks of  $N = 6$ ) has to fulfill that  $\sigma\lambda_2 > \nu_1$  and  $\sigma\lambda_N < \nu_2$ , where  $\sigma$  is the coupling strength and  $\lambda_2$  and  $\lambda_N$  are, respectively, the smallest nonzero eigenvalue and the largest eigenvalue of the Laplacian matrix  $\mathbf{L}$  associated to the *NoN* [17]. If the coupling is introduced through the  $y$  variable (see Eq. S17), the system turns into class II (black circles in Fig. S3). In this case, the synchronization region is determined by the value  $\nu_c = 0.0651$  and the *NoN* only synchronizes for  $\sigma\lambda_2 > \nu_c$ .

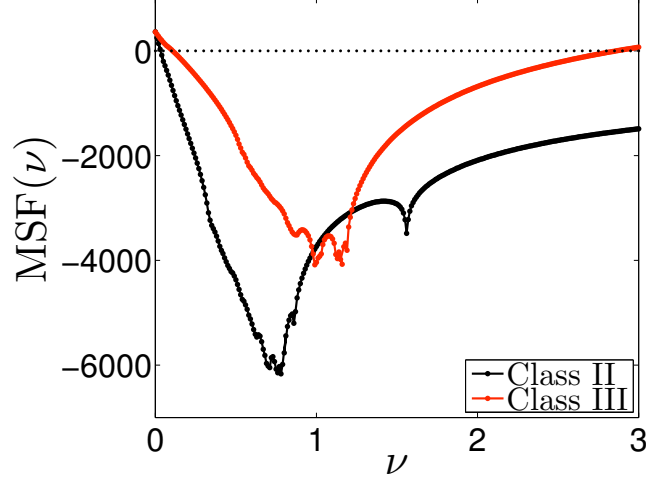

**Figure S3.** (Color online). MSF of Rössler-like oscillators. When the coupling is introduced through the  $x$  variable the system is class III (red circles), while it becomes class II when coupled through the  $y$  variable (black circles). The zeroes of the MSF for the class III and II systems are, respectively,  $\nu_1 = 0.107$  and  $\nu_2 = 2.863$ , and  $\nu_c = 0.0651$ .
